# Supplementary material for: Auto-Pipeline: Synthesizing Complex Data Pipelines By-Target Using Reinforcement Learning and Search
Source: arXiv:2106.13861 source file (2021-08-03)
Supplement: Supplementary file 1 [file appendix.tex]

%!TEX root = main.tex
\appendix
